# Supplementary material for: Mobile-MMLU: A Mobile Intelligence Language Understanding Benchmark
Source: arXiv:2503.20786 source file (2025-03-26)
Supplement: Supplementary file 1 [file appendix.tex]

\section{Some extra stuff}

one, two, three
